# Supplementary material for: Human-AI Collaboration Enables More Empathic Conversations in Text-based Peer-to-Peer Mental Health Support
Source: arXiv:2203.15144 source file (2022-03-28)
Supplement: Supplementary file 1 [file exit-survey-treatment.pdf]

# End-of-study Survey

1) It was **challenging** or **stressful** to write responses to posts.

- Strongly Agree
- Somewhat Agree
- Neutral
- Somewhat Disagree
- Strongly Disagree

2) The **feedback** shown to me was helpful in **improving** my responses.

- Strongly Agree
- Somewhat Agree
- Neutral
- Somewhat Disagree
- Strongly Disagree

3) The **feedback** shown to me was helpful in making my responses more **empathic**.

- Strongly Agree
- Somewhat Agree
- Neutral
- Somewhat Disagree
- Strongly Disagree

4) The **feedback** shown to me was **easy to incorporate** into the final response.

- Strongly Agree
- Somewhat Agree
- Neutral
- Somewhat Disagree
- Strongly Disagree

5) I feel **more confident** at writing supportive responses after this study.

- Strongly Agree
- Somewhat Agree
- Neutral
- Somewhat Disagree
- Strongly Disagree

6) I would like to see this type of feedback system **deployed on TalkLife** or other similar platforms.

- Strongly Agree
- Somewhat Agree
- Neutral
- Somewhat Disagree
- Strongly Disagree

7) Describe the challenges faced while writing responses?

[illegible]

8) Describe instances where feedback was helpful? Why?

9) Describe instances where feedback was not helpful? How could they have been more helpful?

Submit
