# Supplementary material for: Human-AI Collaboration Enables More Empathic Conversations in Text-based Peer-to-Peer Mental Health Support
Source: arXiv:2203.15144 source file (2022-03-28)
Supplement: Supplementary file 2 [file interface-3-treatment.pdf]

## Interface - Insert and Replace Operations

In our feedback, we will **suggest text** that **you can insert or replace** in your current response to make it more supportive and empathic.

### Inserting suggested text

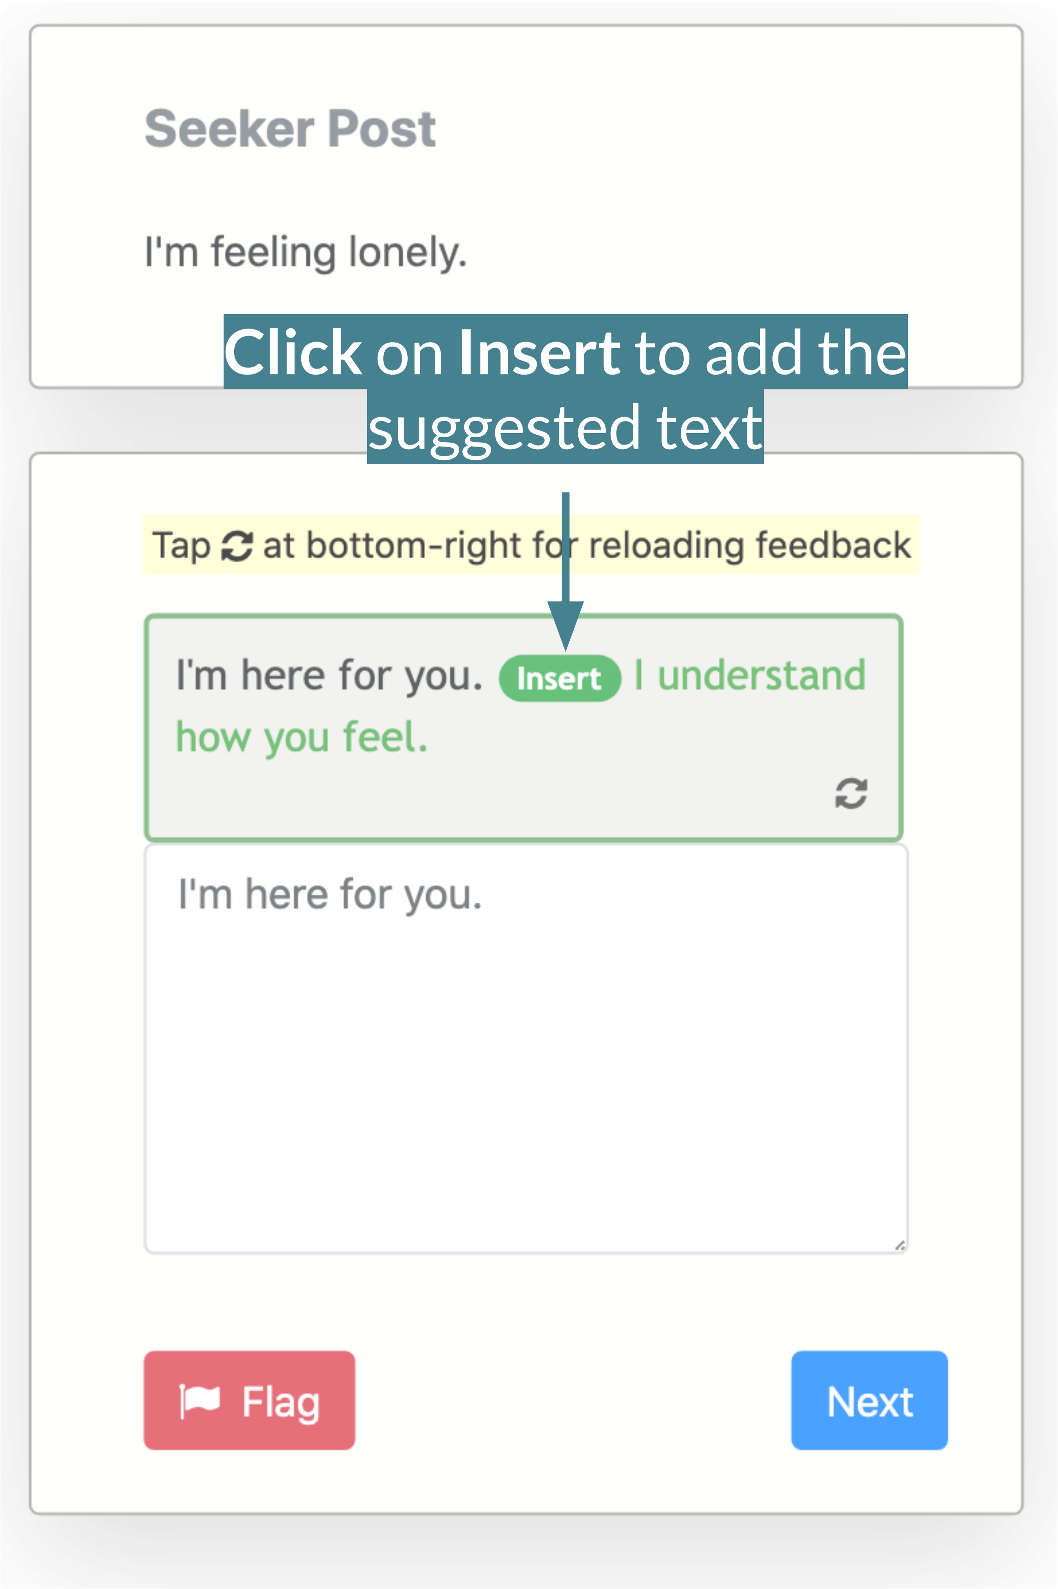

Replacing with suggested text

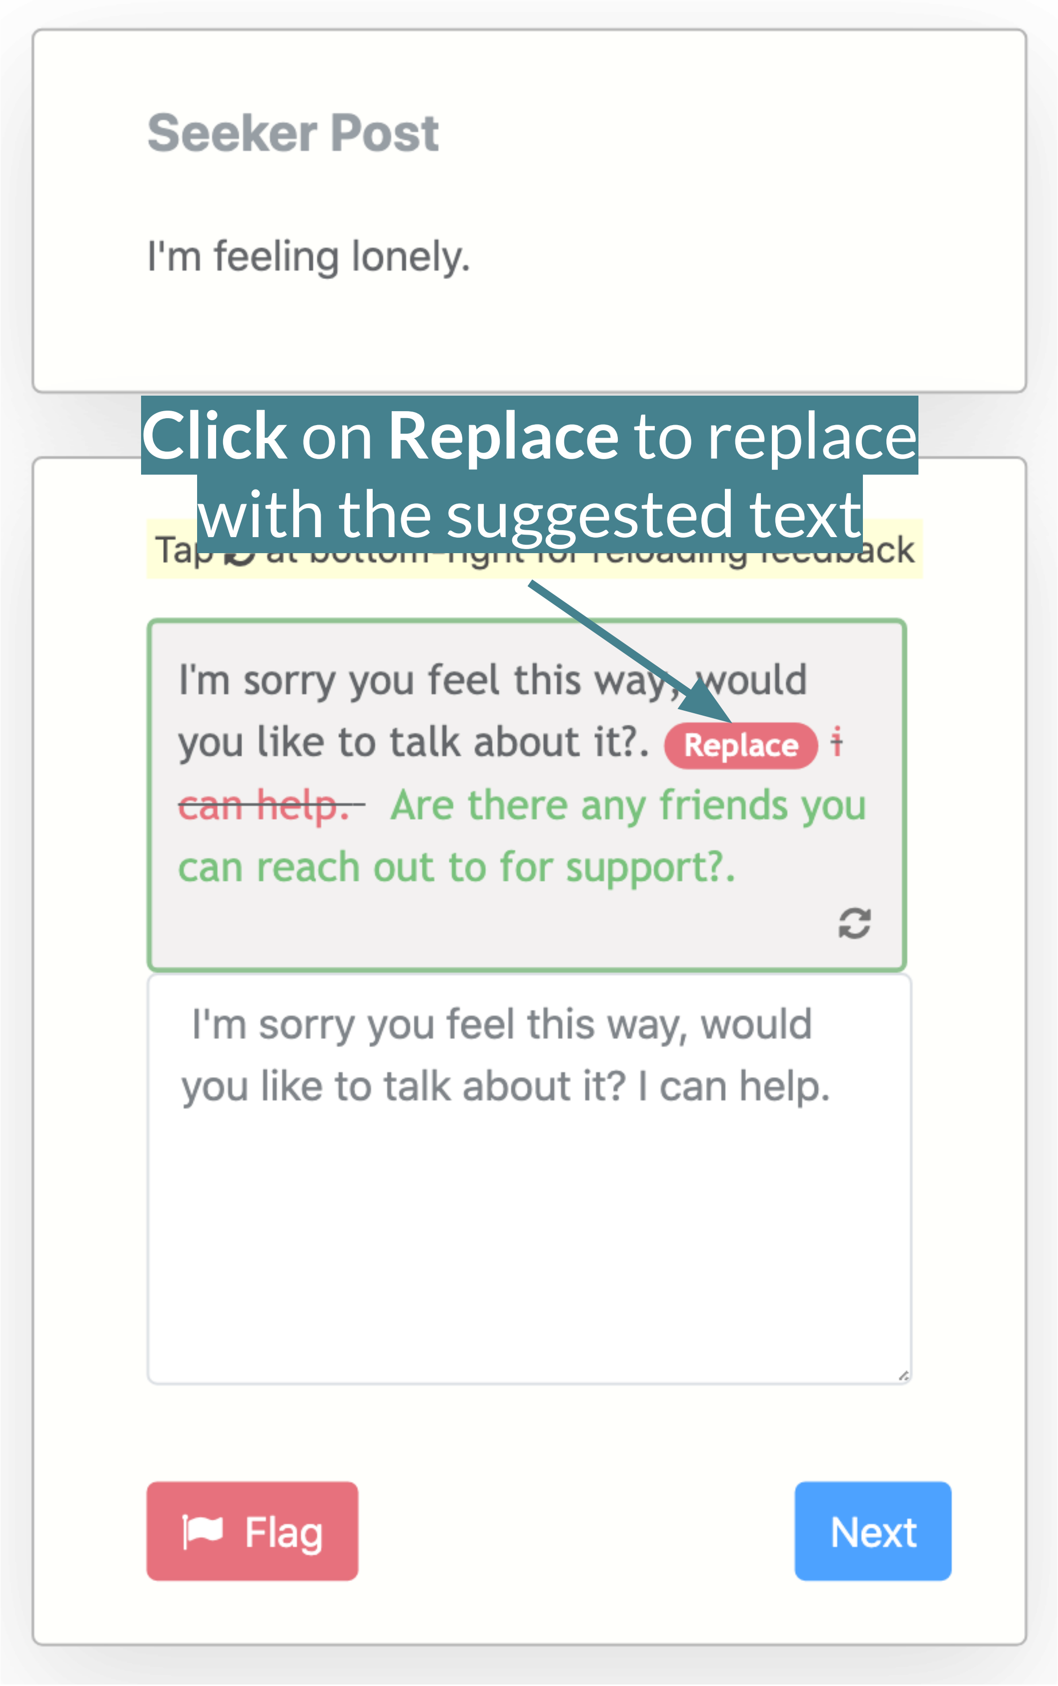


You can directly incorporate the changes by clicking on **Insert** and **Replace** buttons.

Next (3/4)
